# Supplementary material for: Auto-Research Agent on MSA Organization to Improve Protein-Protein Complex Structure Prediction
Source: arXiv:2611.03183 source file (2026-11-03)
Supplement: Supplementary file 1 [file target_level_details.tex]

\section{Target Level Details}
\label{tlD}
% Requires \usepackage{array,booktabs,longtable} in the document preamble.
% Use in a single-column document or appendix; do not wrap in table/table*.
\begingroup
\small
\setlength{\tabcolsep}{5pt}
\renewcommand{\arraystretch}{1.08}
\setlength{\LTcapwidth}{\textwidth}
\begin{longtable}{@{}p{0.33\textwidth}*{5}{>{\raggedleft\arraybackslash}p{\dimexpr0.134\textwidth-2\tabcolsep\relax}}@{}}
\caption{Per-interface results on FBv2: 299 interfaces from 283 targets, grouped by interface type. The experiment contains 2,068 successful submissions in total. Higher DockQ is better.}
\label{tab:fbv2-all-interfaces}\\
\toprule
Interface & Default & \shortstack{Successful\\submissions} & Selection & \multicolumn{2}{c}{Oracle submission} \\
\cmidrule(lr){5-6}
 & DockQ & & DockQ & ID & DockQ \\
\midrule
\endfirsthead
\caption[]{Per-interface results on FBv2 (continued).}\\
\toprule
Interface & Default & \shortstack{Successful\\submissions} & Selection & \multicolumn{2}{c}{Oracle submission} \\
\cmidrule(lr){5-6}
 & DockQ & & DockQ & ID & DockQ \\
\midrule
\endhead
\midrule
\multicolumn{6}{r@{}}{\footnotesize Continued on next page}\\
\endfoot
\bottomrule
\multicolumn{6}{@{}p{\textwidth}@{}}{\footnotesize All scores are mean DockQ over 25 predicted structures (five seeds and five samples per seed), rounded to four decimal places. Default is the first successful native submission (ID 001). The submission count includes Default, counts successful submissions only, and is repeated for interfaces belonging to the same target. Selection is the Agent's final choice. The oracle chooses one successful submission per target by maximizing mean DockQ across that target's interfaces; ties select the earliest submission. All interfaces of a target share this oracle submission, so its score need not be the best for each individual interface. Interface identifiers follow the benchmark's interface IDs.}\\
\endlastfoot
\addlinespace[0.5em]
\multicolumn{6}{@{}l}{\textbf{Homomer-like} ($n=168$ interfaces)}\\*
\texttt{7aal-assembly1\_A\_B} & 0.9344 & 7 & 0.9361 & 004 & 0.9412 \\
\texttt{7bsx-assembly1\_A\_B} & 0.9352 & 6 & 0.9284 & 004 & 0.9394 \\
\texttt{7dnj-assembly1\_A\_B} & 0.6631 & 7 & 0.6532 & 001 & 0.6631 \\
\texttt{7dut-assembly1\_A\_B} & 0.8754 & 8 & 0.9168 & 005 & 0.9168 \\
\texttt{7e1l-assembly1\_A\_B} & 0.3829 & 5 & 0.4388 & 003 & 0.4388 \\
\texttt{7ero-assembly1\_A\_D} & 0.8856 & 6 & 0.8978 & 002 & 0.9133 \\
\texttt{7etr-assembly1\_C\_D} & 0.1066 & 8 & 0.1079 & 006 & 0.1079 \\
\texttt{7etx-assembly1\_A\_B} & 0.6976 & 5 & 0.6976 & 002 & 0.6989 \\
\texttt{7fct-assembly1\_A\_B} & 0.7986 & 5 & 0.8151 & 002 & 0.8186 \\
\texttt{7ff4-assembly1\_A\_B} & 0.4174 & 8 & 0.4174 & 004 & 0.4371 \\
\texttt{7fgq-assembly1\_A\_B} & 0.9282 & 5 & 0.9205 & 002 & 0.9307 \\
\texttt{7kua-assembly1\_A\_B} & 0.8696 & 9 & 0.8628 & 001 & 0.8696 \\
\texttt{7lsc-assembly1\_B\_D} & 0.2636 & 20 & 0.2478 & 003 & 0.5505 \\
\texttt{7n9d-assembly1\_A\_B} & 0.9051 & 4 & 0.9086 & 003 & 0.9124 \\
\texttt{7pcr-assembly1\_A\_B} & 0.4850 & 6 & 0.5944 & 002 & 0.6036 \\
\texttt{7pno-assembly1\_A\_I} & 0.0786 & 8 & 0.0786 & 008 & 0.0844 \\
\texttt{7pyt-assembly1\_B\_D} & 0.7760 & 5 & 0.7822 & 002 & 0.7954 \\
\texttt{7q4i-assembly1\_A\_B} & 0.8701 & 7 & 0.8701 & 003 & 0.8704 \\
\texttt{7qdk-assembly1\_A\_B} & 0.8595 & 9 & 0.8544 & 003 & 0.8768 \\
\texttt{7qtf-assembly1\_B\_C} & 0.8938 & 6 & 0.9145 & 003 & 0.9145 \\
\texttt{7qzo-assembly1\_A\_B} & 0.0214 & 12 & 0.0200 & 004 & 0.0299 \\
\texttt{7rgc-assembly1\_A\_D} & 0.9154 & 5 & 0.9193 & 004 & 0.9205 \\
\texttt{7s2i-assembly1\_A\_B} & 0.8784 & 7 & 0.8671 & 001 & 0.8784 \\
\texttt{7tb5-assembly1\_A\_B} & 0.1880 & 5 & 0.1876 & 002 & 0.1900 \\
\texttt{7tkv-assembly1\_A\_B} & 0.0042 & 9 & 0.0036 & 006 & 0.0055 \\
\texttt{7trw-assembly1\_A\_B} & 0.7669 & 5 & 0.7537 & 002 & 0.7709 \\
\texttt{7tsx-assembly1\_A\_B} & 0.6009 & 6 & 0.6064 & 004 & 0.6087 \\
\texttt{7u7h-assembly1\_A\_B} & 0.8554 & 6 & 0.8551 & 001 & 0.8554 \\
\texttt{7uni-assembly1\_A\_B} & 0.0164 & 5 & 0.0159 & 001 & 0.0164 \\
\texttt{7vb3-assembly1\_A\_B} & 0.8707 & 6 & 0.8635 & 003 & 0.9306 \\
\texttt{7vmh-assembly1\_C\_E} & 0.7582 & 5 & 0.7582 & 004 & 0.7696 \\
\texttt{7voj-assembly1\_A\_B} & 0.8673 & 6 & 0.8674 & 003 & 0.8678 \\
\texttt{7vox-assembly1\_C\_D} & 0.0147 & 7 & 0.0148 & 003 & 0.0151 \\
\texttt{7vqq-assembly1\_A\_B} & 0.0799 & 9 & 0.0857 & 003 & 0.0935 \\
\texttt{7vrx-assembly1\_C\_D} & 0.5779 & 6 & 0.5796 & 004 & 0.5800 \\
\texttt{7vwk-assembly1\_A\_B} & 0.8372 & 6 & 0.8372 & 004 & 0.8424 \\
\texttt{7w07-assembly1\_A\_B} & 0.0040 & 10 & 0.4354 & 007 & 0.4539 \\
\texttt{7wdq-assembly1\_A\_B} & 0.8563 & 5 & 0.8455 & 001 & 0.8563 \\
\texttt{7wm6-assembly1\_A\_B} & 0.9485 & 7 & 0.9482 & 005 & 0.9693 \\
\texttt{7xoz-assembly1\_A\_D} & 0.2487 & 12 & 0.0477 & 003 & 0.4119 \\
\texttt{7y73-assembly1\_A\_B} & 0.8044 & 6 & 0.8044 & 002 & 0.8046 \\
\texttt{7yul-assembly1\_A\_C} & 0.1517 & 5 & 0.1426 & 003 & 0.1814 \\
\texttt{7zcv-assembly1\_A\_B} & 0.6359 & 9 & 0.6797 & 009 & 0.7083 \\
\texttt{8a2g-assembly1\_A\_B} & 0.1551 & 6 & 0.1551 & 002 & 0.2998 \\
\texttt{8a8g-assembly1\_A\_B} & 0.4566 & 7 & 0.4597 & 003 & 0.4665 \\
\texttt{8a8q-assembly1\_C\_D} & 0.1956 & 5 & 0.1956 & 001 & 0.1956 \\
\texttt{8aid-assembly1\_A\_B} & 0.9161 & 6 & 0.9140 & 003 & 0.9182 \\
\texttt{8am6-assembly1\_A\_B} & 0.9351 & 10 & 0.9434 & 010 & 0.9518 \\
\texttt{8apr-assembly1\_A\_B} & 0.9621 & 5 & 0.9621 & 004 & 0.9650 \\
\texttt{8axr-assembly1\_A\_C} & 0.9660 & 3 & 0.9660 & 003 & 0.9720 \\
\texttt{8azc-assembly1\_A\_B} & 0.0246 & 6 & 0.0324 & 004 & 0.0338 \\
\texttt{8bey-assembly1\_A\_B} & 0.0404 & 8 & 0.0407 & 005 & 0.0407 \\
\texttt{8bwd-assembly1\_A\_B} & 0.7837 & 10 & 0.7636 & 010 & 0.7919 \\
\texttt{8cid-assembly1\_A\_B} & 0.6568 & 9 & 0.7953 & 003 & 0.7997 \\
\texttt{8cil-assembly1\_A\_B} & 0.5336 & 7 & 0.5423 & 007 & 0.5711 \\
\texttt{8cjw-assembly1\_A\_B} & 0.3590 & 7 & 0.3568 & 007 & 0.3607 \\
\texttt{8cjw-assembly1\_A\_C} & 0.3787 & 7 & 0.3806 & 007 & 0.3844 \\
\texttt{8cra-assembly1\_A\_B} & 0.6626 & 9 & 0.6872 & 009 & 0.6882 \\
\texttt{8d0p-assembly1\_A\_B} & 0.9048 & 7 & 0.9048 & 006 & 0.9145 \\
\texttt{8dfb-assembly1\_A\_B} & 0.0328 & 6 & 0.0554 & 004 & 0.0554 \\
\texttt{8ee7-assembly1\_A\_B} & 0.6159 & 7 & 0.6230 & 007 & 0.6230 \\
\texttt{8eht-assembly1\_A\_B} & 0.6748 & 9 & 0.8728 & 004 & 0.8728 \\
\texttt{8enq-assembly1\_D\_E} & 0.0267 & 7 & 0.0267 & 001 & 0.0267 \\
\texttt{8fw7-assembly1\_C\_O} & 0.0128 & 7 & 0.0126 & 005 & 0.0538 \\
\texttt{8g01-assembly1\_B\_C} & 0.0192 & 18 & 0.0274 & 012 & 0.0492 \\
\texttt{8g02-assembly1\_E\_F} & 0.0160 & 11 & 0.0533 & 010 & 0.0704 \\
\texttt{8gci-assembly1\_A\_B} & 0.9395 & 5 & 0.9274 & 001 & 0.9395 \\
\texttt{8gps-assembly1\_A\_B} & 0.4334 & 5 & 0.8858 & 004 & 0.8858 \\
\texttt{8gro-assembly1\_A\_B} & 0.3218 & 7 & 0.3249 & 003 & 0.3279 \\
\texttt{8h3z-assembly1\_A\_B} & 0.8756 & 11 & 0.8883 & 011 & 0.8901 \\
\texttt{8h8p-assembly1\_A\_B} & 0.7810 & 7 & 0.7736 & 005 & 0.7925 \\
\texttt{8hr5-assembly1\_A\_B} & 0.4516 & 9 & 0.5762 & 005 & 0.5762 \\
\texttt{8hvq-assembly1\_A\_B} & 0.1250 & 5 & 0.1900 & 002 & 0.1900 \\
\texttt{8i3c-assembly1\_A\_B} & 0.8406 & 5 & 0.8410 & 002 & 0.8415 \\
\texttt{8i3x-assembly1\_A\_B} & 0.6311 & 5 & 0.7052 & 002 & 0.7052 \\
\texttt{8ioo-assembly1\_A\_B} & 0.8483 & 5 & 0.8483 & 003 & 0.8525 \\
\texttt{8je0-assembly1\_A\_D} & 0.9349 & 7 & 0.9216 & 004 & 0.9361 \\
\texttt{8k25-assembly1\_C\_D} & 0.0224 & 8 & 0.0318 & 003 & 0.0419 \\
\texttt{8k74-assembly1\_A\_B} & 0.9680 & 6 & 0.9680 & 003 & 0.9690 \\
\texttt{8kdk-assembly1\_A\_B} & 0.7907 & 7 & 0.8488 & 005 & 0.8570 \\
\texttt{8p0s-assembly1\_A\_B} & 0.5836 & 8 & 0.5848 & 002 & 0.5862 \\
\texttt{8pe0-assembly1\_A\_B} & 0.0313 & 11 & 0.0420 & 006 & 0.0420 \\
\texttt{8phb-assembly1\_A\_B} & 0.5698 & 5 & 0.5698 & 001 & 0.5698 \\
\texttt{8q0e-assembly1\_A\_B} & 0.8963 & 10 & 0.9001 & 005 & 0.9206 \\
\texttt{8q57-assembly1\_A\_C} & 0.8584 & 9 & 0.8730 & 009 & 0.8801 \\
\texttt{8qlh-assembly1\_A\_B} & 0.0069 & 8 & 0.0065 & 004 & 0.0078 \\
\texttt{8ron-assembly1\_A\_B} & 0.7431 & 6 & 0.7392 & 005 & 0.7534 \\
\texttt{8rst-assembly1\_A\_C} & 0.6635 & 6 & 0.6550 & 001 & 0.6635 \\
\texttt{8rxb-assembly1\_E\_G} & 0.0197 & 5 & 0.0209 & 005 & 0.0244 \\
\texttt{8sde-assembly1\_A\_B} & 0.0276 & 9 & 0.0480 & 009 & 0.0654 \\
\texttt{8sdi-assembly1\_B\_D} & 0.7658 & 7 & 0.7926 & 003 & 0.8109 \\
\texttt{8sm8-assembly1\_A\_B} & 0.9232 & 6 & 0.9061 & 001 & 0.9232 \\
\texttt{8t0w-assembly1\_A\_B} & 0.9492 & 5 & 0.9421 & 001 & 0.9492 \\
\texttt{8t5y-assembly1\_A\_B} & 0.6914 & 9 & 0.6503 & 001 & 0.6914 \\
\texttt{8tcs-assembly1\_A\_B} & 0.9132 & 7 & 0.9146 & 003 & 0.9194 \\
\texttt{8u0n-assembly1\_A\_B} & 0.9159 & 5 & 0.9162 & 004 & 0.9280 \\
\texttt{8u1a-assembly1\_A\_B} & 0.0056 & 6 & 0.0056 & 002 & 0.0059 \\
\texttt{8u8m-assembly1\_A\_B} & 0.0165 & 6 & 0.0942 & 005 & 0.0942 \\
\texttt{8ur2-assembly1\_A\_C} & 0.8920 & 4 & 0.8928 & 003 & 0.8942 \\
\texttt{8uvk-assembly1\_A\_B} & 0.7742 & 8 & 0.7241 & 001 & 0.7742 \\
\texttt{8v4g-assembly1\_A\_B} & 0.9348 & 4 & 0.9377 & 002 & 0.9377 \\
\texttt{8vxb-assembly1\_A\_B} & 0.9048 & 5 & 0.9072 & 003 & 0.9091 \\
\texttt{8weu-assembly1\_A\_B} & 0.8585 & 8 & 0.8616 & 008 & 0.8630 \\
\texttt{8wto-assembly1\_A\_B} & 0.3572 & 8 & 0.3625 & 008 & 0.3625 \\
\texttt{8wwd-assembly1\_A\_B} & 0.7926 & 5 & 0.8938 & 005 & 0.8938 \\
\texttt{8wws-assembly1\_A\_B} & 0.8870 & 6 & 0.8870 & 006 & 0.8916 \\
\texttt{8xh7-assembly1\_A\_C} & 0.0620 & 7 & 0.0102 & 002 & 0.1294 \\
\texttt{8xha-assembly1\_A\_B} & 0.6946 & 9 & 0.7248 & 007 & 0.7307 \\
\texttt{8xpf-assembly1\_A\_C} & 0.6185 & 5 & 0.6185 & 003 & 0.7579 \\
\texttt{8xte-assembly1\_A\_B} & 0.6590 & 5 & 0.6989 & 005 & 0.6989 \\
\texttt{8y7p-assembly1\_A\_B} & 0.9262 & 10 & 0.9411 & 003 & 0.9436 \\
\texttt{8yel-assembly1\_A\_B} & 0.5629 & 8 & 0.5426 & 001 & 0.5629 \\
\texttt{8yel-assembly1\_A\_C} & 0.5618 & 8 & 0.5416 & 001 & 0.5618 \\
\texttt{8ylh-assembly1\_A\_B} & 0.7070 & 5 & 0.7077 & 004 & 0.7077 \\
\texttt{8z6d-assembly1\_A\_B} & 0.7779 & 5 & 0.7883 & 002 & 0.8077 \\
\texttt{8z6e-assembly1\_A\_B} & 0.9074 & 4 & 0.9074 & 002 & 0.9347 \\
\texttt{8zaz-assembly1\_A\_B} & 0.0094 & 9 & 0.0055 & 009 & 0.0192 \\
\texttt{8zxk-assembly1\_A\_C} & 0.9562 & 6 & 0.9562 & 001 & 0.9562 \\
\texttt{8zxk-assembly1\_B\_C} & 0.9647 & 6 & 0.9647 & 001 & 0.9647 \\
\texttt{9b2f-assembly1\_A\_B} & 0.9066 & 8 & 0.9066 & 002 & 0.9166 \\
\texttt{9b4p-assembly1\_A\_C} & 0.4326 & 22 & 0.6899 & 016 & 0.6899 \\
\texttt{9b6c-assembly1\_A\_B} & 0.6691 & 6 & 0.6691 & 005 & 0.6872 \\
\texttt{9bce-assembly1\_A\_B} & 0.8318 & 7 & 0.8318 & 002 & 0.8445 \\
\texttt{9bou-assembly1\_A\_B} & 0.8261 & 8 & 0.8386 & 004 & 0.8393 \\
\texttt{9bua-assembly1\_A\_B} & 0.8428 & 10 & 0.8695 & 010 & 0.8860 \\
\texttt{9c9q-assembly1\_A\_B} & 0.7489 & 7 & 0.7572 & 005 & 0.7600 \\
\texttt{9cck-assembly1\_A\_B} & 0.7783 & 7 & 0.8872 & 005 & 0.8872 \\
\texttt{9ebm-assembly1\_A\_B} & 0.7674 & 9 & 0.9247 & 009 & 0.9247 \\
\texttt{9f7o-assembly1\_A\_B} & 0.8872 & 5 & 0.8900 & 003 & 0.8938 \\
\texttt{9fdo-assembly1\_A\_B} & 0.0279 & 14 & 0.0264 & 005 & 0.0301 \\
\texttt{9fkr-assembly1\_A\_B} & 0.0045 & 10 & 0.0041 & 003 & 0.0176 \\
\texttt{9fm7-assembly1\_A\_B} & 0.7565 & 5 & 0.7620 & 002 & 0.8224 \\
\texttt{9fo7-assembly1\_A\_B} & 0.2886 & 7 & 0.4262 & 004 & 0.4264 \\
\texttt{9gzg-assembly1\_A\_B} & 0.0140 & 7 & 0.0143 & 007 & 0.0148 \\
\texttt{9h8j-assembly1\_B\_D} & 0.7160 & 15 & 0.6813 & 007 & 0.7189 \\
\texttt{9hh1-assembly1\_A\_B} & 0.9770 & 5 & 0.9770 & 001 & 0.9770 \\
\texttt{9hmy-assembly1\_A\_B} & 0.4278 & 7 & 0.4352 & 003 & 0.4394 \\
\texttt{9hqb-assembly1\_A\_C} & 0.3389 & 8 & 0.3160 & 005 & 0.4762 \\
\texttt{9htx-assembly1\_B\_D} & 0.7090 & 8 & 0.7256 & 004 & 0.7653 \\
\texttt{9if9-assembly1\_C\_A} & 0.0404 & 8 & 0.0716 & 006 & 0.1131 \\
\texttt{9ikv-assembly1\_A\_B} & 0.8006 & 6 & 0.8805 & 004 & 0.8805 \\
\texttt{9iqw-assembly1\_A\_D} & 0.5670 & 14 & 0.6324 & 005 & 0.6335 \\
\texttt{9jn6-assembly1\_A\_B} & 0.9028 & 4 & 0.9028 & 001 & 0.9028 \\
\texttt{9k2j-assembly1\_A\_B} & 0.9074 & 6 & 0.9074 & 002 & 0.9280 \\
\texttt{9kea-assembly1\_C\_D} & 0.9058 & 7 & 0.8616 & 006 & 0.9421 \\
\texttt{9kl2-assembly1\_A\_B} & 0.3840 & 5 & 0.3840 & 005 & 0.7925 \\
\texttt{9kpr-assembly1\_A\_B} & 0.7017 & 7 & 0.7065 & 006 & 0.7076 \\
\texttt{9le4-assembly1\_B\_D} & 0.0206 & 10 & 0.0298 & 006 & 0.0696 \\
\texttt{9lil-assembly1\_A\_B} & 0.7501 & 6 & 0.6484 & 001 & 0.7501 \\
\texttt{9m7c-assembly1\_A\_B} & 0.7856 & 10 & 0.7864 & 003 & 0.7886 \\
\texttt{9m7c-assembly1\_A\_F} & 0.7966 & 10 & 0.7980 & 003 & 0.8034 \\
\texttt{9mgh-assembly1\_A\_C} & 0.3416 & 11 & 0.8183 & 007 & 0.8183 \\
\texttt{9mgh-assembly1\_A\_D} & 0.7620 & 11 & 0.9036 & 007 & 0.9036 \\
\texttt{9mkr-assembly1\_A\_B} & 0.6416 & 9 & 0.7682 & 004 & 0.7813 \\
\texttt{9no2-assembly1\_B\_D} & 0.7594 & 7 & 0.8056 & 007 & 0.8137 \\
\texttt{9o5w-assembly1\_A\_B} & 0.7446 & 8 & 0.9094 & 007 & 0.9128 \\
\texttt{9olu-assembly1\_A\_B} & 0.8271 & 6 & 0.7817 & 001 & 0.8271 \\
\texttt{9ps2-assembly1\_A\_B} & 0.0208 & 10 & 0.0472 & 010 & 0.1136 \\
\texttt{9qky-assembly1\_B\_E} & 0.0211 & 7 & 0.0260 & 007 & 0.0265 \\
\texttt{9qtp-assembly1\_C\_D} & 0.9609 & 4 & 0.9609 & 001 & 0.9609 \\
\texttt{9rxh-assembly1\_A\_B} & 0.4453 & 10 & 0.5294 & 005 & 0.5937 \\
\texttt{9sp7-assembly1\_A\_B} & 0.5777 & 6 & 0.5812 & 006 & 0.5812 \\
\texttt{9ubq-assembly1\_A\_D} & 0.0198 & 10 & 0.4634 & 006 & 0.4834 \\
\texttt{9ugs-assembly1\_A\_B} & 0.8041 & 8 & 0.7882 & 002 & 0.8183 \\
\texttt{9w1n-assembly1\_A\_B} & 0.0052 & 6 & 0.0090 & 005 & 0.0090 \\
\texttt{9x7g-assembly1\_A\_B} & 0.0088 & 9 & 0.0088 & 004 & 0.0088 \\
\texttt{9y12-assembly1\_A\_B} & 0.9215 & 5 & 0.9215 & 005 & 0.9246 \\
\texttt{9y5y-assembly1\_J\_L} & 0.0379 & 10 & 0.0345 & 003 & 0.0613 \\
\addlinespace[0.5em]
\multicolumn{6}{@{}l}{\textbf{Same-species heteromer} ($n=100$ interfaces)}\\*
\texttt{7fc0-assembly1\_A\_B} & 0.3122 & 5 & 0.3238 & 005 & 0.3241 \\
\texttt{7ffn-assembly1\_A\_E} & 0.5567 & 7 & 0.5768 & 005 & 0.6262 \\
\texttt{7lb8-assembly1\_A\_D} & 0.6691 & 8 & 0.6777 & 006 & 0.6777 \\
\texttt{7n00-assembly1\_A\_C} & 0.8068 & 7 & 0.8068 & 002 & 0.8484 \\
\texttt{7n40-assembly1\_A\_B} & 0.8434 & 5 & 0.8434 & 004 & 0.9180 \\
\texttt{7o0y-assembly1\_A\_D} & 0.6318 & 10 & 0.6422 & 003 & 0.6434 \\
\texttt{7olh-assembly1\_B\_C} & 0.4876 & 8 & 0.5154 & 005 & 0.5341 \\
\texttt{7p1n-assembly1\_A\_B} & 0.9074 & 6 & 0.9120 & 004 & 0.9161 \\
\texttt{7p4a-assembly1\_A\_B} & 0.7479 & 10 & 0.8284 & 009 & 0.8288 \\
\texttt{7pb8-assembly1\_B\_D} & 0.7579 & 6 & 0.7579 & 003 & 0.7627 \\
\texttt{7pyt-assembly1\_A\_D} & 0.7495 & 5 & 0.8212 & 002 & 0.8186 \\
\texttt{7q5n-assembly1\_B\_D} & 0.0194 & 12 & 0.0183 & 008 & 0.0260 \\
\texttt{7qv0-assembly1\_A\_L} & 0.7446 & 7 & 0.7603 & 006 & 0.7661 \\
\texttt{7sf7-assembly1\_A\_B} & 0.7232 & 8 & 0.7236 & 007 & 0.7236 \\
\texttt{7tcx-assembly1\_A\_B} & 0.8334 & 5 & 0.8641 & 002 & 0.8671 \\
\texttt{7tqd-assembly1\_A\_C} & 0.8390 & 7 & 0.8597 & 003 & 0.8648 \\
\texttt{7uv8-assembly1\_A\_C} & 0.2052 & 4 & 0.2313 & 002 & 0.2352 \\
\texttt{7v8l-assembly1\_A\_B} & 0.0521 & 5 & 0.0326 & 005 & 0.0807 \\
\texttt{7vru-assembly1\_A\_B} & 0.4581 & 10 & 0.4270 & 002 & 0.5516 \\
\texttt{7xoi-assembly1\_A\_B} & 0.8502 & 4 & 0.8502 & 002 & 0.8704 \\
\texttt{7xva-assembly1\_A\_B} & 0.6221 & 5 & 0.7099 & 003 & 0.7130 \\
\texttt{7y64-assembly1\_E\_F} & 0.7924 & 4 & 0.7908 & 004 & 0.7968 \\
\texttt{7yjo-assembly1\_C\_E} & 0.8733 & 5 & 0.8733 & 003 & 0.9017 \\
\texttt{7yls-assembly1\_A\_B} & 0.8810 & 7 & 0.8880 & 007 & 0.8882 \\
\texttt{7z36-assembly1\_A\_D} & 0.7766 & 6 & 0.7766 & 004 & 0.8251 \\
\texttt{7zdt-assembly1\_A\_B} & 0.4486 & 8 & 0.4490 & 005 & 0.4598 \\
\texttt{8ap8-assembly1\_A\_D} & 0.8063 & 6 & 0.8108 & 006 & 0.8330 \\
\texttt{8ap8-assembly1\_C\_D} & 0.7914 & 6 & 0.8323 & 006 & 0.8457 \\
\texttt{8b3j-assembly1\_A\_C} & 0.7598 & 6 & 0.7598 & 003 & 0.7829 \\
\texttt{8b3j-assembly1\_B\_C} & 0.7119 & 6 & 0.7119 & 003 & 0.7281 \\
\texttt{8b4a-assembly1\_A\_C} & 0.1132 & 12 & 0.0907 & 007 & 0.1300 \\
\texttt{8blw-assembly1\_A\_B} & 0.6606 & 8 & 0.6360 & 002 & 0.6819 \\
\texttt{8bwl-assembly1\_A\_D} & 0.7834 & 7 & 0.7785 & 001 & 0.7834 \\
\texttt{8dgq-assembly1\_A\_B} & 0.2284 & 11 & 0.4344 & 007 & 0.4344 \\
\texttt{8do6-assembly1\_C\_H} & 0.7379 & 8 & 0.7178 & 002 & 0.7634 \\
\texttt{8dps-assembly1\_B\_C} & 0.8359 & 6 & 0.8219 & 002 & 0.8432 \\
\texttt{8ebb-assembly1\_A\_B} & 0.7869 & 5 & 0.9427 & 005 & 0.9427 \\
\texttt{8esd-assembly1\_A\_B} & 0.7199 & 4 & 0.7199 & 001 & 0.7199 \\
\texttt{8esd-assembly1\_A\_D} & 0.8921 & 4 & 0.8921 & 001 & 0.8921 \\
\texttt{8ffu-assembly1\_A\_B} & 0.8977 & 6 & 0.9182 & 002 & 0.9182 \\
\texttt{8gqe-assembly1\_A\_B} & 0.7686 & 7 & 0.8681 & 007 & 0.8859 \\
\texttt{8hhj-assembly1\_A\_B} & 0.6922 & 6 & 0.6900 & 002 & 0.8050 \\
\texttt{8hi1-assembly1\_D\_E} & 0.9003 & 11 & 0.8674 & 004 & 0.9027 \\
\texttt{8hk0-assembly1\_A\_C} & 0.9019 & 4 & 0.8941 & 001 & 0.9019 \\
\texttt{8j5d-assembly1\_A\_C} & 0.8280 & 6 & 0.8571 & 004 & 0.8571 \\
\texttt{8j5d-assembly1\_B\_C} & 0.8193 & 6 & 0.8465 & 004 & 0.8465 \\
\texttt{8j9n-assembly1\_A\_B} & 0.2036 & 9 & 0.2427 & 005 & 0.3252 \\
\texttt{8kgg-assembly1\_A\_E} & 0.6620 & 10 & 0.6868 & 005 & 0.7048 \\
\texttt{8ou0-assembly1\_B\_C} & 0.0050 & 9 & 0.0115 & 009 & 0.0115 \\
\texttt{8ouz-assembly1\_B\_C} & 0.7596 & 9 & 0.7606 & 008 & 0.7674 \\
\texttt{8ouz-assembly1\_C\_D} & 0.8698 & 9 & 0.8642 & 008 & 0.8761 \\
\texttt{8ows-assembly1\_A\_B} & 0.7960 & 5 & 0.7960 & 004 & 0.8418 \\
\texttt{8p1u-assembly1\_B\_C} & 0.3566 & 6 & 0.3540 & 001 & 0.3566 \\
\texttt{8pjn-assembly1\_A\_C} & 0.7544 & 7 & 0.7738 & 005 & 0.7759 \\
\texttt{8qat-assembly1\_A\_C} & 0.3240 & 11 & 0.1425 & 001 & 0.3240 \\
\texttt{8qat-assembly1\_A\_D} & 0.6632 & 11 & 0.5980 & 001 & 0.6632 \\
\texttt{8qbn-assembly1\_A\_C} & 0.8000 & 7 & 0.8622 & 007 & 0.8622 \\
\texttt{8qvc-assembly1\_A\_D} & 0.7492 & 6 & 0.7679 & 003 & 0.7955 \\
\texttt{8qvd-assembly1\_B\_C} & 0.9125 & 9 & 0.9250 & 008 & 0.9287 \\
\texttt{8s02-assembly1\_A\_B} & 0.8996 & 7 & 0.8939 & 006 & 0.9116 \\
\texttt{8sjj-assembly1\_A\_B} & 0.7219 & 5 & 0.7119 & 002 & 0.7399 \\
\texttt{8ttb-assembly1\_C\_D} & 0.4079 & 15 & 0.6426 & 011 & 0.6426 \\
\texttt{8tz0-assembly1\_A\_E} & 0.9095 & 7 & 0.8362 & 001 & 0.9095 \\
\texttt{8tzr-assembly1\_A\_C} & 0.0128 & 6 & 0.0196 & 004 & 0.0376 \\
\texttt{8u8c-assembly1\_A\_D} & 0.8293 & 3 & 0.8293 & 003 & 0.8359 \\
\texttt{8v2a-assembly1\_A\_B} & 0.7332 & 6 & 0.7382 & 003 & 0.7387 \\
\texttt{8wdb-assembly1\_A\_B} & 0.5488 & 6 & 0.5614 & 005 & 0.5646 \\
\texttt{8wvy-assembly1\_A\_B} & 0.0356 & 6 & 0.7506 & 006 & 0.7506 \\
\texttt{8xu0-assembly1\_A\_B} & 0.6710 & 6 & 0.6658 & 004 & 0.6726 \\
\texttt{8xup-assembly1\_A\_E} & 0.7151 & 8 & 0.7151 & 004 & 0.7703 \\
\texttt{8xup-assembly1\_B\_E} & 0.4986 & 8 & 0.4986 & 004 & 0.6515 \\
\texttt{8xyp-assembly1\_C\_D} & 0.9148 & 7 & 0.9089 & 001 & 0.9148 \\
\texttt{8yn0-assembly1\_A\_C} & 0.2642 & 8 & 0.3477 & 002 & 0.4207 \\
\texttt{8zh8-assembly1\_A\_G} & 0.7486 & 12 & 0.7513 & 010 & 0.7519 \\
\texttt{8zue-assembly1\_A\_B} & 0.6837 & 4 & 0.7141 & 004 & 0.7141 \\
\texttt{9bt4-assembly1\_C\_D} & 0.0040 & 7 & 0.0040 & 001 & 0.0040 \\
\texttt{9d0x-assembly1\_A\_C} & 0.0065 & 7 & 0.0063 & 004 & 0.0071 \\
\texttt{9dlp-assembly1\_A\_B} & 0.9188 & 5 & 0.9188 & 001 & 0.9188 \\
\texttt{9dur-assembly1\_A\_B} & 0.0281 & 8 & 0.0293 & 003 & 0.0293 \\
\texttt{9e03-assembly1\_A\_B} & 0.3395 & 7 & 0.6515 & 003 & 0.6515 \\
\texttt{9e8p-assembly1\_A\_B} & 0.0109 & 8 & 0.0109 & 005 & 0.0166 \\
\texttt{9fn0-assembly1\_A\_B} & 0.9087 & 6 & 0.9244 & 006 & 0.9244 \\
\texttt{9gtu-assembly1\_B\_C} & 0.1956 & 6 & 0.2076 & 005 & 0.2086 \\
\texttt{9gwj-assembly1\_C\_D} & 0.7429 & 5 & 0.7429 & 001 & 0.7429 \\
\texttt{9h6e-assembly1\_A\_B} & 0.6990 & 5 & 0.7784 & 004 & 0.8013 \\
\texttt{9hac-assembly1\_A\_B} & 0.4623 & 6 & 0.4233 & 001 & 0.4623 \\
\texttt{9hbk-assembly1\_B\_D} & 0.2962 & 9 & 0.5550 & 007 & 0.5550 \\
\texttt{9his-assembly1\_B\_D} & 0.6320 & 8 & 0.8164 & 006 & 0.8251 \\
\texttt{9i3u-assembly1\_A\_C} & 0.0123 & 16 & 0.0086 & 003 & 0.0359 \\
\texttt{9k27-assembly1\_A\_F} & 0.7593 & 7 & 0.7509 & 001 & 0.7593 \\
\texttt{9ko4-assembly1\_A\_B} & 0.6759 & 6 & 0.5690 & 001 & 0.6759 \\
\texttt{9kx6-assembly1\_A\_D} & 0.6316 & 8 & 0.6316 & 003 & 0.6349 \\
\texttt{9m08-assembly1\_A\_C} & 0.7207 & 10 & 0.7242 & 009 & 0.7431 \\
\texttt{9mj5-assembly1\_B\_D} & 0.2722 & 9 & 0.2655 & 001 & 0.2722 \\
\texttt{9myr-assembly1\_A\_B} & 0.9372 & 4 & 0.9414 & 004 & 0.9429 \\
\texttt{9mza-assembly1\_A\_D} & 0.0223 & 6 & 0.0151 & 005 & 0.0262 \\
\texttt{9n49-assembly1\_C\_F} & 0.1356 & 11 & 0.2780 & 007 & 0.2983 \\
\texttt{9nh1-assembly1\_A\_D} & 0.0048 & 6 & 0.1029 & 005 & 0.1352 \\
\texttt{9qa5-assembly1\_A\_B} & 0.8904 & 5 & 0.8958 & 002 & 0.8972 \\
\texttt{9w9h-assembly1\_A\_B} & 0.6477 & 7 & 0.6260 & 002 & 0.6489 \\
\addlinespace[0.5em]
\multicolumn{6}{@{}l}{\textbf{Cross-species} ($n=31$ interfaces)}\\*
\texttt{7evp-assembly1\_A\_D} & 0.0660 & 5 & 0.0808 & 004 & 0.0808 \\
\texttt{7evp-assembly1\_B\_C} & 0.0656 & 5 & 0.0809 & 004 & 0.0809 \\
\texttt{7ffn-assembly1\_C\_D} & 0.1221 & 7 & 0.6310 & 005 & 0.6403 \\
\texttt{7jrd-assembly1\_B\_A} & 0.0040 & 7 & 0.0040 & 006 & 0.0049 \\
\texttt{7yld-assembly1\_A\_B} & 0.1266 & 8 & 0.1266 & 001 & 0.1266 \\
\texttt{7z73-assembly1\_A\_F} & 0.3014 & 9 & 0.0581 & 004 & 0.5806 \\
\texttt{8a47-assembly1\_A\_C} & 0.4402 & 8 & 0.4402 & 001 & 0.4402 \\
\texttt{8a60-assembly1\_A\_B} & 0.0089 & 6 & 0.0062 & 002 & 0.0103 \\
\texttt{8cis-assembly1\_A\_B} & 0.0971 & 6 & 0.2186 & 002 & 0.2186 \\
\texttt{8cxj-assembly1\_A\_B} & 0.9021 & 4 & 0.9016 & 001 & 0.9021 \\
\texttt{8eia-assembly1\_B\_C} & 0.8442 & 7 & 0.8449 & 007 & 0.8456 \\
\texttt{8enk-assembly1\_A\_C} & 0.7949 & 5 & 0.7949 & 004 & 0.8002 \\
\texttt{8fvj-assembly1\_B\_J} & 0.0109 & 10 & 0.0066 & 002 & 0.0165 \\
\texttt{8gti-assembly1\_A\_B} & 0.0049 & 15 & 0.0183 & 012 & 0.0183 \\
\texttt{8s1x-assembly1\_A\_B} & 0.3168 & 7 & 0.2841 & 001 & 0.3168 \\
\texttt{8tcg-assembly1\_A\_C} & 0.8814 & 6 & 0.8814 & 001 & 0.8814 \\
\texttt{8tcg-assembly1\_B\_C} & 0.8608 & 6 & 0.8608 & 001 & 0.8608 \\
\texttt{8uro-assembly1\_A\_B} & 0.3649 & 7 & 0.6068 & 007 & 0.6288 \\
\texttt{8yat-assembly1\_B\_D} & 0.1109 & 11 & 0.1083 & 005 & 0.1406 \\
\texttt{9bt8-assembly1\_A\_E} & 0.0280 & 9 & 0.0280 & 003 & 0.0355 \\
\texttt{9e55-assembly1\_B\_C} & 0.5655 & 5 & 0.5655 & 001 & 0.5655 \\
\texttt{9fdy-assembly1\_C\_E} & 0.4962 & 8 & 0.5147 & 002 & 0.5444 \\
\texttt{9fe1-assembly1\_A\_D} & 0.0235 & 7 & 0.0235 & 004 & 0.0271 \\
\texttt{9hb3-assembly1\_A\_E} & 0.4194 & 8 & 0.4977 & 004 & 0.4977 \\
\texttt{9hiz-assembly1\_A\_C} & 0.8551 & 10 & 0.8553 & 007 & 0.8868 \\
\texttt{9l99-assembly1\_B\_E} & 0.0082 & 5 & 0.0082 & 003 & 0.0353 \\
\texttt{9l9a-assembly1\_D\_E} & 0.1615 & 5 & 0.1615 & 001 & 0.1615 \\
\texttt{9oc6-assembly1\_A\_C} & 0.1838 & 7 & 0.9032 & 007 & 0.9032 \\
\texttt{9q1h-assembly1\_A\_B} & 0.8546 & 10 & 0.8574 & 005 & 0.8747 \\
\texttt{9r5y-assembly1\_A\_B} & 0.0614 & 11 & 0.1034 & 010 & 0.1064 \\
\texttt{9u94-assembly1\_A\_D} & 0.0194 & 6 & 0.0194 & 003 & 0.0366 \\
\end{longtable}
\endgroup
